# Supplementary material for: Deep Learning Applied to Chest X-Rays: Exploiting and Preventing Shortcuts
Source: arXiv:2009.10132 source file (2020-09-21)
Supplement: Supplementary file 1 [file appendix.tex]

\begin{table*}[h]
    \centering
    \caption{\label{tab:skewed_unskewed_datasets} We resampled the unskewed training set such that it was comparable in size to the skewed training set. To mimic the test set distribution, there was no correlation between CHF and each attribute in the unskewed training set. On the other hand, there was a 1:1 correlation between CHF and each attribute in the skewed training set.}
\scalebox{0.85}{
\begin{tabular}{c c c c c}
\toprule
\textbf{Attribute} & \multicolumn{2}{c}{\textbf{Unskewed Training Set}} & \multicolumn{2}{c}{\textbf{Skewed Training Set}} \\ & \textbf{N Train (\%)} & \textbf{N Valid (\%)} &  \textbf{N Train (\%)} & \textbf{N Valid (\%)}  \\ 
 \midrule
\textbf{BMI} &  $477$ $(0.10)$ & $119$ $(0.12)$ & $508$ $(0.12)$ & $127$ $(0.13)$ \\
\textbf{Age} &  $508$ $(0.21)$ & $129$ $(0.26)$ & $553$ $(0.25)$ & $139$ $(0.19)$ \\
\textbf{Sex} &  $457$ $(0.10)$ & $114$ $(0.10)$ & $504$ $(0.12)$ & $127$ $(0.10)$ \\

\textbf{Race} & $644$ $(0.02)$ & $157$ $(0.03)$ & $706$ $(0.01)$ & $177$ $(0.02)$ \\ 
\textbf{Pacemaker} &  $785$ $(0.06)$ & $192$ $(0.07)$ & $780$ $(0.06)$ & $195$ $(0.06)$ \\

 \bottomrule
\end{tabular}
}
\end{table*}

\begin{table*}[h]
    \centering
    \caption{\label{tab:assumption_datasets} We vary the amount of correlation between pneumonia and BMI, ranging from -1 to 1 in increments of 0.5. We aimed to keep the training and validation sets similar in size as well as prevalence of pneumonia, so as to not give one training set an advantage over another.}
\scalebox{0.85}{
\begin{tabular}{c c c c c c c}
\toprule
\textbf{Correlation} & \textbf{-1.0} & \textbf{-0.5} &  \textbf{0} &  \textbf{0.5} & \textbf{1.0} \\ 
 \midrule
\textbf{N Train (\%)} & $465$ $(0.27)$ & $478$ $(0.21)$ & $483$ $(0.23)$ & $481$ $(0.21)$ & $486$ $(0.25)$  \\
 \textbf{N Valid (\%)} & $114$ $(0.26)$ & $122$ $(0.30)$ & $117$ $(0.23)$ & $119$ $(0.18)$ & $125$ $(0.18)$ \\
 
 \bottomrule
\end{tabular}
}
\end{table*}

\begin{table*}[h]
    \centering
    \caption{\label{tab:statistical_tests_us} Statistical significance of the improvement in performance of the model trained on an unskewed dataset vs. a model trained on a skewed datset. The model trained on an unskewed dataset performs statistically better for BMI, sex, and race.}
\scalebox{0.85}{
\begin{tabular}{ c c}
\toprule
& \textbf{p-value} \\ 
 \midrule
\textbf{BMI} & 0.03 \\
\textbf{Age} & 0.20 \\
\textbf{Sex} & 0.02 \\
\textbf{Race} & 0.00 \\
\textbf{Pacemaker} & 0.70 \\
 \bottomrule
\end{tabular}
}
\end{table*}

\begin{table*}[h]
    \centering
    \caption{\label{tab:statistical_tests} Statistical significance of the improvement in performance of the single task approach vs. the transfer learning approach. The model trained on an unskewed dataset performs statistically better for BMI and race.}
\scalebox{0.85}{
\begin{tabular}{ c c}
\toprule
& \textbf{p-value} \\ 
 \midrule
\textbf{BMI} & 0.03 \\
\textbf{Age} & 0.15 \\
\textbf{Sex} & 0.25 \\
\textbf{Race} & 0.00 \\
\textbf{Pacemaker} & 0.20 \\
 \bottomrule
\end{tabular}
}
\end{table*}
